# Supplementary material for: AnyVIO: Feed-Forward Streaming Visual-Inertial Odometry Across Platforms
Source: arXiv:2611.26625 source file (2026-11-19)
Supplement: Supplementary file 1 [file X_suppl.tex]

\clearpage
\setcounter{page}{1}
\maketitlesupplementary


\section{Implementation details}\label{sec:method:visual:appendix}
Details on nominal parameters used in the visual backbone, imu encoder, and fusion module are in Tab~\ref{tab:nominalparams}.

\subsection{Visual Backbone Training Losses}
%We start from the released \VGGTO~\cite{wang2026vggt} weights with new mask and scale heads. 
We fine-tune the causal backbone and both heads jointly on windows of $\SubmapSize=16$ frames. 
%The objective is the original \VGGTO and VGGT loss~\cite{wang2026vggt,wang2025vggt} on the cameras, depth and points in scene-normalised units, a binary cross-entropy on the mask logits (with weight $0.03$) and two metric terms on each of the $\SubmapSize-1$ edges. 
The loss is defined as in~\cite{wang2026vggt,wang2025vggt} for cameras, depth, and points in scene-normalized units. To this, we add a binary cross-entropy on the mask logits and two metric %terms on each of the $\SubmapSize-1$ edges. 
terms for each pair of consecutive camera poses.
\iffalse
Let $\Delta\bar{\Position}_{\FrameIndex}$ be the predicted step of edge $\FrameIndex$ in scene-normalised units and $\Delta\Position_{\FrameIndex}$ the true metric step. The first term regresses $\SubmapLogScale_{\WindowIndex,\FrameIndex}$ to the least-squares log scale $\log\big(\Delta\bar{\Position}_{\FrameIndex}^{\Transpose}\Delta\Position_{\FrameIndex}/\|\Delta\bar{\Position}_{\FrameIndex}\|^2\big)$ (the target is not backpropagated). The second term penalises the relative step error
\begin{equation}
\frac{\SubmapScale_{\WindowIndex,\FrameIndex}\Delta\bar{\Position}_{\FrameIndex}-\Delta\Position_{\FrameIndex}}{\max(\|\Delta\Position_{\FrameIndex}\|,\,0.1\,\text{m})},
\end{equation}
which normalises slow and fast motion. Both use a Huber loss with threshold $0.1$, skip steps less than $1$\,cm, and backprop into the backbone. The camera regressor and scale head are then fine-tuned on the cached features with trajectory losses over longer training periods. This also allows for the use of datasets which have ground-truth poses but no dense depth.
\fi 
 %The first term regresses $\SubmapLogScale_{\WindowIndex,\FrameIndex}$ to the least-squares log scale $\log\big(\Delta\bar{\Position}_{\FrameIndex}^{\Transpose}\Delta\Position_{\FrameIndex}/\|\Delta\bar{\Position}_{\FrameIndex}\|^2\big)$ (the target is not backpropagated). The second term penalises the relative step error
Specifically, we define a loss
\begin{align*}
    \mathcal{L}_S =& \sum_{k,i}H_{\delta}\Big(\hspace{-2pt}{\lambda_{k,i} -} \log\Big(\hspace{-2pt}\frac{\Delta\bar{\Position}_{\FrameIndex}^{\Transpose}\Delta\Position_{\FrameIndex}}{\|\Delta\bar{\Position}_{\FrameIndex}\|^2}\hspace{-2pt}\Big)\hspace{-2pt}\Big) + \\ &\sum_{k,i}H_{\delta}\Big(\frac{{\|e^{\lambda_{k,i}}}\Delta\bar{\Position}_{\FrameIndex}-\Delta\Position_{\FrameIndex}{\|}}{\max(\|\Delta\Position_{\FrameIndex}\|,\,0.1)}\hspace{-1pt}
    \Big)
\end{align*}
where $H_{\delta}$ is the Huber loss with threshold $\delta$. The first term regresses $\SubmapLogScale_{\WindowIndex,\FrameIndex}$ to the least-squares log scale, while the second directly trains scale and the predicted displacement.

\section{IMU Implementation}

\noindent\textbf{Velocity normalization.}
For a sample $n$ from dataset $d$, the scale in~\eqref{eq:imu_velocity_loss} is
\begin{equation}\label{eq:app:imu_scale}
\begin{aligned}
c_n&=\min\!\Big(\sigma_d,\ \sqrt{\|\mathbf v^B_n\|+v_0}\Big),\\
\sigma_d&=\max\!\Big(\sqrt{\tfrac13\textstyle\sum_{a}s_{d,a}^2},\ \sigma_{\min}\Big),
\end{aligned}
\end{equation}
where $s_{d,a}$ is the standard deviation of the training velocities of dataset $d$ along axis $a$, $\sigma_{\min}=0.25$\,m/s, and $v_0=0.5$\,m/s. The dataset scale $\sigma_d$ is shared by all three axes. Per-axis scaling would otherwise divide the forward error of driving data by its large spread and thereby down-weight the axis that matters most. The speed term $\sqrt{\|\mathbf v^B_n\|+v_0}$ replaces $\sigma_d$ whenever it is smaller, so errors at low speed on fast platforms are not discounted. $v_0$ keeps it positive at standstill.

\mg{Maybe comment on the projection done to convert the tacked visual and geometric features into the GRU input. I think these are jointly projected through a weight matrix, a bias is added, and they're passed through some activation function. We could include an equation of this somewhere here.}

\begin{table}[t]
    \centering
    \caption{Nominal parameters}
    \begin{tabular}{c c c}
    \toprule
    & Parameter & Value \\\midrule
     \multirow{4}{*}{\rotatebox[origin=c]{90}{Sec.~\ref{sec:method:streamingvisual}}} & $\SubmapSize$ & 16 \\
    & $H_u$ & 128 \\
    & $\SubmapLogScale_0$   &  ?\\
    & $\SubmapLogScale_c$  &  12\\
       \bottomrule
    \end{tabular}
    \label{tab:nominalparams}
\end{table}

\section{Hardware details}\label{app:harwaredetails}

\section{Self collected Dataset Construction}


%\subsection{\ourdataset}
\label{sec:data:race}
\setlength{\columnsep}{8pt}
\begin{wrapfigure}{r}{0.4\columnwidth}
\vspace{-10pt}

\includegraphics[width=0.4\columnwidth]{filled_data_distribution/motion_filled.pdf}
\vspace{-24pt}

\caption{Sets containing 99\% of data distributions.}
\label{fig:data:motion}
\end{wrapfigure}
%Open-source driving datasets are dominated by feature-rich urban scenes, and rarely incorporate motions with large simultaneous attitude rates and velocity. 
To evaluate odometry under more extreme motion and noisy visual measurements, we collected a \ourdataset dataset with two test vehicles at a racing facility (see~\cref{fig:mosaic}),  
%The \texttt{tarmac} vehicle is driven on a 2-mile asphalt race track at 
including high speeds asphalt runs $\|\boldsymbol{v}\|>40$ m/s %. The \texttt{off-road} vehicle is driven 
and aggressive off-road  runs% on a 0.6-mile dirt course,
 with large sideslip\footnote{Sideslip is defined as $\beta = \arctan(v_y^B/v_x^B)$ with velocities expressed in a vehicle-fixed frame, see e.g.,~\cite{djeumou2024one}.} exceeding $ 50^\circ$ (which is higher than typical drifting maneuvers~\cite{djeumou2024one}), higher attitude rates $\|\boldsymbol{\omega}\|>1.3$ rad/s, and strong chassis vibrations affecting the IMU noise levels. %This extends the range of camera speed and angular speed well beyond public driving datasets (see~\cref{fig:data:motion}).
\ourdataset differs visually from most driving datasets~\cite{DBLP:journals/corr/abs-1903-11027,geiger2013vision,Liao2022PAMI,sivaprakasam2024tartandrive}. The scenes are open and repetitive, with few nearby features, a large sky regions, and frequent glare, which is difficult for most odometry methods (\cref{tab:draft:driving:ape}). In the off-road setting, there are clouds of dust that, together with haze, can obscure the scene almost entirely (\cref{fig:OODtrajectories}).

% collapse that donw...

Each recording contains unrectified images from a forward-facing camera (29Hz, 1440x928, {\color{red}WFOVxHFOV}), IMU measurements (501 Hz), LiDAR scans (10Hz) for depth supervision, and ground-truth poses from an OxTS RTK GPS/INS~\cite{oxts2026} (62.5 Hz).  We split recordings from various lighting and weather conditions into training, validation, and test sets (see~\cref{tab:datasets}), and hold out recordings from on-board deployments with poor lighting, reverse laps, and dust occlusion (see~\cref{sec:hwresults}.).
\newpage\section{Hardware Results}\label{app:harware}

\subsection{Data mix}\label{app:harware:data}
\mg{I believe we only used the models generated prior to the trip on Odin, not sure what mix you used in Leia in the end. Maybe we should refer to the appendix and include details?}
\oa{Yes will clarify this in the appendix, its a mix that has nothing from october for testing for Odin, and for Leia we updated the training split with runs from the previous day given the new imu calibration}

\subsection{Hardware details}\label{app:harware:details}

\subsection{Additional Results}\label{app:harware:additional}
\mg{These results are probably not needed, and some might not make sense to include depending on how we structure the paper. I'll add them here for now. They include:
\begin{itemize}
    \item An ablation on stride and CAN usage in HW (see Tab.~\ref{tab:ablateStrideInHardware}). Using stride 3 generally seems better; CAN can be used, but then we start to drop frames. It is about as good as the VIO in the few tests that we ran on the car. This motivated our use of stride=3 and no CAN, which we have kept throughout the experiment section.
    \item A comparison of reverse laps in Leia with good/bad lighting (see Tab.~\ref{tab:ablateCWgoodbadlighting}). Here, the results are a bit mixed and inconclusive -- we actually have better metrics in the poor lighting setting across the board, but they are very close. Clearly, it seems that we are more sensitive to driving in the reverse direction than to changing lighting conditions with this model; we had different drivers in the two tests, so the driving style will have differed. To me, it would make sense to include these results if we want to establish what works worse in the OOD setting, switching the direction to CW or dimming the light. However, I do not think we have enough data/evidence to study this properly, and would suggest omitting these results.
\end{itemize}

}

\begin{table}[htbp]
    \caption{On-vehicle results, \textbf{in-distribution} \texttt{offroad} setting. Ablating the stride parameter in the ROS node and the use of CAN signals in the fusion module. Runs $\{068, 069\}$ are a bit slower and less crazy than $\{072,072\}$ and therefore have lower VO metrics. Based on these results, we ran the rest of the experiments on Wednesday with stride 3 (improvement in VIO) and without CAN (marginal benefit + slower).}
    \vspace{-7pt}
    \centering
    \resizebox{\columnwidth}{!}{\begin{tabular}{l|c|c|c|cc|cc|c}\toprule
         \tabheader{Method} & \tabheader{Stride} & \tabheader{Use CAN} & \tabheader{Exp.} & \multicolumn{2}{c|}{\tabheader{RPE (per 100m)}} & \multicolumn{2}{c|}{\tabheader{APE (m)}} & \tabheader{FPS (Hz)} \\
         & & & &Trans. & Rot. & SE(3) & Sim(3) \\\midrule
         \ourmethod-VO & 2 & \xmark& 068 & 3.29 & 1.67 & 9.72 & 9.26 & 10.23 \\
         \ourmethod-VIO  & 2 & \xmark & 068 & 3.39 & 1.04 & 6.34 & 5.50 & 10.23 \\
         \ourmethod-VO & 3 & \xmark& 069 &  3.57 & 1.54 & 6.17 & 5.60 & 10.20 \\
         \ourmethod-VIO  & 3 & \xmark& 069 & 2.77 & 0.85 & 3.76 & 3.06 & 10.20\\\midrule
          \ourmethod-VO  & 3 & \xmark& 072 & 4.12 & 1.68 & 10.53 & 10.38 & 10.02 \\
         \ourmethod-VIO & 3 & \xmark& 072 & 3.22 & 1.04 & 6.72 & 6.06 & 10.02 \\
          \ourmethod-VO  & 3 & \xmark& 075 & 5.04 & 1.86 & 7.66& 6.91 & 7.47 \\
         \ourmethod-VIO & 3 & \cmark& 075 & 4.37 & 0.81 & 6.51 & 6.45 & 7.47 \\
         \bottomrule
    \end{tabular}}
    \label{tab:ablateStrideInHardware}
\end{table}


\begin{table}[htbp]
    \caption{On-car results in \textbf{out-of-distribution} settings with aggressive driving, reverse laps, \textbf{poor vs. good lighting}.}
    \vspace{-7pt}
    \label{tab:metricsOODDboth}
    \centering
    \resizebox{\columnwidth}{!}{\begin{tabular}{l|c|cc|cc|c}\toprule
         \tabheader{Method} & \tabheader{Exp.} & \multicolumn{2}{c|}{\tabheader{RPE (per 100m)}} & \multicolumn{2}{c|}{\tabheader{APE (m)}} & \tabheader{FPS (Hz)} \\
         & & Trans. & Rot. & SE(3) & Sim(3) \\ \bottomrule\toprule
         \multicolumn{7}{c}{\texttt{tarmac} (max speed $>32$ m/s, max sideslip $>4^{\circ}$, CW, \textbf{good lighting})}\\\midrule
         Tartan-IMU & 187 &  24.34& 21.88 &97.85&94.12&20.01 \\
         \ourmethod-VO& 187 & 6.08&1.51&27.52&18.56&9.79 \\
         \ourmethod-VIO & 187 & 4.90&1.21&26.71&16.62&9.79 \\ \bottomrule\toprule
         \multicolumn{7}{c}{\texttt{tarmac} (max speed $>32$ m/s, max sideslip $>4^{\circ}$, CW, \textbf{poor lighting})}\\\midrule
         Tartan-IMU & 217 &  24.80 & 20.71 & 98.52 & 84.52 & 20.01 \\
         \ourmethod-VO& 217 &4.87 & 1.45 & 17.70 & 13.38 & 9.75 \\
         \ourmethod-VIO & 217 & 4.41 & 1.18 & 19.93 & 12.20 & 9.75 \\\bottomrule
    \end{tabular}}
    \label{tab:ablateCWgoodbadlighting}
\end{table}



\begin{table}[htbp]

\caption{\textbf{Fusion ablation averaged over all evaluated datasets.} Equal-weight means of dataset averages: 11 datasets (70 recordings, 88 segments) for APE; nine datasets with eligible 100\,m intervals for RPE. APE is position RMSE (m); RPE is translation drift (\%) and rotation drift ($^\circ$/100\,m). Lower is better. Completed-submap head rollouts use frozen causal experts. Constant trust uses validation-selected $(w_t,w_r)=(0.1,0.7)$; learned corrections, visual rescaling and fusion state are retained, without retraining.}
\label{tab:ablation:fusion}
\centering\scriptsize\setlength{\tabcolsep}{3pt}
\resizebox{0.75\columnwidth}{!}{%
\begin{tabular}{@{}lrrrr@{}}\toprule
 & \multicolumn{2}{c}{APE (m)} & \multicolumn{2}{c}{RPE (100\,m)} \\
Variant & SE(3) & Sim(3) & Trans. (\%) & Rot. ($^\circ$) \\ \midrule
VO & 11.19 & 8.13 & 5.48 & 6.77 \\
VO + blind twin & 11.12 & 7.93 & 5.40 & 6.32 \\
Constant trust & 6.88 & 4.37 & 4.67 & 2.95 \\
Adaptive trust & \textbf{5.86} & \textbf{3.48} & \textbf{4.55} & \textbf{2.61} \\
\bottomrule\end{tabular}}
\end{table}





\section{Rationale}
\label{sec:rationale}
% 
Having the supplementary compiled together with the main paper means that:
% 
\begin{itemize}
\item The supplementary can back-reference sections of the main paper, for example, we can refer to \cref{sec:intro};
\item The main paper can forward reference sub-sections within the supplementary explicitly (e.g. referring to a particular experiment); 
\item When submitted to arXiv, the supplementary will already included at the end of the paper.
\end{itemize}
% 
To split the supplementary pages from the main paper, you can use \href{https://support.apple.com/en-ca/guide/preview/prvw11793/mac#:~:text=Delete%20a%20page%20from%20a,or%20choose%20Edit%20%3E%20Delete).}{Preview (on macOS)}, \href{https://www.adobe.com/acrobat/how-to/delete-pages-from-pdf.html#:~:text=Choose%20%E2%80%9CTools%E2%80%9D%20%3E%20%E2%80%9COrganize,or%20pages%20from%20the%20file.}{Adobe Acrobat} (on all OSs), as well as \href{https://superuser.com/questions/517986/is-it-possible-to-delete-some-pages-of-a-pdf-document}{command line tools}.

% @misc{shen2025fastvggttrainingfreeaccelerationvisual,
%       title={FastVGGT: Training-Free Acceleration of Visual Geometry Transformer}, 
%       author={You Shen and Zhipeng Zhang and Yansong Qu and Xiawu Zheng and Jiayi Ji and Shengchuan Zhang and Liujuan Cao},
%       year={2025},
%       eprint={2509.02560},
%       archivePrefix={arXiv},
%       primaryClass={cs.CV},
%       url={https://arxiv.org/abs/2509.02560}, 
% }
